# Supplementary material for: Zero-shot Neural Transfer for Cross-lingual Entity Linking
Source: arXiv:1811.04154 source file (2018-11-09)
Supplement: Supplementary file 1 [file supplementary.tex]

\begin{table*}[tb]
% \small
\centering
\renewcommand{\arraystretch}{1.05}
%\resizebox{\textwidth}{!}{
\begin{tabular}{@{}ll|ccccccccc@{}}
% \toprule
  Model &  In. & bn & jv & lo & mr & pa & te & ti & uk & ug\\ \midrule
  \textbf{\textsc{Exact}} & 
  G &  .00 & .63 & .02 & .00 & .00 & .00 & .02 & .02 & .03 \\
  
  \textbf{\textsc{Trans}} & 
  G &  .00 & .63 & .02 & .17 & .00 & .00 & .46 & .02 & .03 \\ \midrule
  \textbf{\textsc{Encode}}  & &  \\
  \multirow{3}{*}{\textsc{Manual}} 
  & G & .00 & .70 & .02 & .46 & .00 & .00 & .40 & .25 & .06 \\
  & P  & .36 & .66 & .04 & .41 & .11 & .06 & .44 & .04 & .11 \\
  & A & .32 & .65 & .07 & .37 & .31 & .20 & .37 & .12 & .16 \\
  \cmidrule{3-11}
   \multirow{3}{*}{\textsc{Best-55}} 
   & G & .00 & .70 & .03 (de) & .46 & .00 & .00 & .40 & .41 (kk) & .09 (ckb)\\
  & P & .38 (ms) & .68 (yo) & .06 (hi) & .41 & .13 (te) & .3 (hi) & .44 & .21 (pl) & .16 (am)\\
  & A & .34 (ms) & .66 (hi) & .07 & .37 & .36 (te) & .36 (pa) & .37  & .23 (hi) & .16 \\
  \cmidrule{3-11}
    \multirow{3}{*}{\textsc{Unwt}} & G &
    \\
  & P &  \\
  & A &   \\
  \cmidrule{3-11}
   \multirow{3}{*}{\textsc{WtComb}} & G &
  \\
  & P &   \\
  & A &  \\ 
  \midrule
  \textbf{\textsc{Pivot}} & & \\
  \multirow{3}{*}{\textsc{Manual}} 
  & G & .00 & .86 & .02 & .62 & .00 & .00 & .61 & .50 & .08 \\
  & P & .48 & .84 & .20 & .58 & .18 & .10 & .69 & .23 & .21 \\
  & A & .45 & .82 & .28 & .56 & .49 & .33 & .63 & .42 & .29 \\
  \cmidrule{3-11}
   \multirow{3}{*}{\textsc{Best-55}} 
   & G & .00 & .86 & .03 (jv) & .62 & .00 & .00 & .61 & .54 (kk) & .12 (ckb) \\
  & P & .48 & .84 & .20 & .58 & .18 & .38 (hi) & .69 & .30 (pl) & .23 (am) \\
  & A &  .48 (mr) & .82 & .28 & .56 & .49 & .47 (hi) & .63 & .42 & .32 \\
  \cmidrule{3-11}
    \multirow{3}{*}{\textsc{UnwtComb}} & G &
   \\
  & P &  \\
  & A &   \\
  \cmidrule{3-11}
   \multirow{3}{*}{\textsc{WtComb}} & G &
   \\
  & P &   \\
  & A &  \\ 
  \midrule
  
  
\end{tabular}
%}
\caption{Entity linking accuracy with \textbf{G}rapheme, \textbf{P}honeme or \textbf{A}rticulary features as input.}
\label{table: wiki}
\end{table*}
